# Supplementary material for: Orbital magneto-optical response of periodic insulators from first principles
Source: arXiv:1806.09886 ancillary file (2019-02-25)
Supplement: Supplementary file 1 [file SI.pdf]

# Supplementary information for “Orbital magneto-optical response of periodic insulators from first principles”

Irina V. Lebedeva,<sup>1,\*</sup> David A. Strubbe,<sup>2</sup> Ilya V. Tokatly,<sup>1,3,4</sup> and Angel Rubio<sup>1,5,†</sup>

<sup>1</sup>*Nano-Bio Spectroscopy Group and ETSF, Departamento de Física de Materiales, Universidad del País Vasco UPV/EHU, 20018 San Sebastián, Spain*

<sup>2</sup>*Department of Physics, School of Natural Sciences, University of California, Merced, CA, 95343, United States*

<sup>3</sup>*Donostia International Physics Center (DIPC), Manuel de Lardizabal 5, 20018 San Sebastián, Spain*

<sup>4</sup>*IKERBASQUE, Basque Foundation for Science, 48011 Bilbao, Spain*

<sup>5</sup>*Max Planck Institute for the Structure and Dynamics of Matter and Center for Free-Electron Laser Science, Luruper Chaussee 149, 22761 Hamburg, Germany*

## CONTENTS

|                                                          |   |
|----------------------------------------------------------|---|
| 1. Adiabatic local-field effects                         | 1 |
| 2. Solid-state formulation                               | 1 |
| 2.1. General form of equations                           | 1 |
| 2.2. First-order derivatives of the density matrix       | 2 |
| 2.3. Second-order derivatives of the density matrix      | 2 |
| 2.4. Polarizability in the absence of the magnetic field | 3 |
| 2.5. Band magnetic dipole moments                        | 4 |
| 3. Finite-system formulation                             | 4 |
| 3.1. Equations solved                                    | 4 |
| 3.2. $\mathcal{A}$ and $\mathcal{B}$ terms               | 4 |
| 4. Angle of Faraday rotation and ellipticity             | 5 |
| 5. Additional details and results of calculations        | 6 |
| 5.1. k-point grids and local-field effects               | 6 |
| 5.2. Valley g-factor from tight-binding model            | 7 |
| 5.3. Computational time                                  | 7 |
| References                                               | 8 |

## 1. ADIABATIC LOCAL-FIELD EFFECTS

In the independent particle picture, the periodic part of the Hamiltonian is the same as the Hamiltonian in the absence of the external field  $\tilde{H} = H_0$  and does not depend on the perturbation  $P$ . To take into account particle interactions, corrections to the Hartree, exchange and correlation terms are included:  $\partial\tilde{H}/\partial P = U_{\text{Hxc}}^{(1)}[n^{(P)}] + U_{\text{xc}}^{(2)}[n^{(P)}, n^{(P)}]$ . These terms arise from the derivative of the electron density  $n^{(P)}(\mathbf{r}) = \rho^{(P)}(\mathbf{r}, \mathbf{r}')\delta(\mathbf{r} - \mathbf{r}')$  to the perturbation  $P$  and to the second order in  $n^{(P)}$  and in the adiabatic approximation are given by

$$U_{\text{Hxc}}^{(1)} = \int f_{\text{Hxc}}(\mathbf{r}, \mathbf{r}') n^{(P)}(\mathbf{r}') d\mathbf{r}', \quad (1)$$

$$U_{\text{xc}}^{(2)} = \frac{1}{2} \int K_{\text{xc}}(\mathbf{r}, \mathbf{r}', \mathbf{r}'') n^{(P)}(\mathbf{r}') n^{(P)}(\mathbf{r}'') d\mathbf{r}' d\mathbf{r}'', \quad (2)$$

where  $f_{\text{Hxc}}$  and  $K_{\text{xc}}$  are the adiabatic kernels related to the exchange-correlation potential  $v_{\text{xc}}$  as

$$f_{\text{Hxc}}[n^{(0)}](\mathbf{r}, \mathbf{r}') = \left. \frac{\delta v_{\text{xc}}(\mathbf{r})}{\delta n(\mathbf{r}')} \right|_{n=n^{(0)}} + \frac{1}{|\mathbf{r} - \mathbf{r}'|} \quad (3)$$

and

$$K_{\text{xc}}[n^{(0)}](\mathbf{r}, \mathbf{r}', \mathbf{r}'') = \left. \frac{\delta^2 v_{\text{xc}}(\mathbf{r})}{\delta n(\mathbf{r}') \delta n(\mathbf{r}'')} \right|_{n=n^{(0)}}. \quad (4)$$

It should be noted that the change in the electron density is zero for  $k \cdot p$  perturbations<sup>1</sup>. Furthermore, in systems with time-reversal symmetry in the ground state, the change of the electron density should also comply with time-reversal symmetry and for the first order in the magnetic field, it is possible only when the change in the electron density is zero. This is the case for all the systems considered in the present paper.

## 2. SOLID-STATE FORMULATION

### 2.1. General form of equations

For solids, it is convenient to work with equations in reciprocal space. We, therefore, represent the operators as (note that we omit tilde in reciprocal space)

$$\tilde{\mathcal{O}}_{\mathbf{r}_1 \mathbf{r}_2} = \int_{\text{BZ}} \frac{d\mathbf{k}}{(2\pi)^3} e^{i\mathbf{k}\mathbf{r}_1} \mathcal{O}_{\mathbf{k}} e^{-i\mathbf{k}\mathbf{r}_2}. \quad (5)$$

In reciprocal space, Eq. (15) of the paper corresponding to the Liouville equation projected onto unperturbed Kohn-Sham states can be written as

$$\mathcal{L}_{v\mathbf{k}}(\Omega) |\zeta_{v\mathbf{k}}^{(P)}\rangle = P_{c\mathbf{k}} \mathcal{R}^{(P)} [\rho_{\mathbf{k}}^{(n-1)}, \dots, \rho_{\mathbf{k}}^{(0)}, n^{(P)}] |u_{v\mathbf{k}}^{(0)}\rangle, \quad (6)$$

where  $\mathcal{L}_{v\mathbf{k}}(\Omega) = \Omega + H_{0\mathbf{k}} - \epsilon_{v\mathbf{k}}$ ,  $\mathcal{R}^{(P)} = R_{\mathbf{k}}^{(P)}$ ,  $|u_{v\mathbf{k}}^{(0)}\rangle$  and  $|\zeta_{v\mathbf{k}}^{(P)}\rangle$  are the periodic parts of wavefunctions  $|\eta_{v\mathbf{k}}^{(P)}\rangle = e^{i\mathbf{k}\mathbf{r}} |\zeta_{v\mathbf{k}}^{(P)}\rangle$  and  $|\psi_{v\mathbf{k}}^{(0)}\rangle = e^{i\mathbf{k}\mathbf{r}} |u_{v\mathbf{k}}^{(0)}\rangle$ , respectively, and  $P_{c\mathbf{k}} = 1 - P_{v\mathbf{k}} = 1 - \rho_{\mathbf{k}}^{(0)}$  is the projector onto unoccupied bands at k-point  $\mathbf{k}$ .

As mentioned in the paper, there is no need to solve the Liouville equation for the block diagonal elements  $\tilde{\rho}_D^{(P)}$  of the derivative of the density matrix within occupied ( $\tilde{\rho}_{VV}^{(P)} = -P_v \tilde{\rho}_D^{(P)} P_v$ ) and unoccupied ( $\tilde{\rho}_{CC}^{(P)} = P_c \tilde{\rho}_D^{(P)} P_c$ ) subspaces. These can be found explicitly from the idempotency condition for the Kohn-Sham density matrix  $\rho = \rho\rho$  (Refs. 2 and 3), which to the first order in the magnetic field is given by Eq. (18) of the paper. In terms of the block diagonal part of the density matrix in reciprocal space,  $\rho_{\mathbf{k}D} = (1 - \rho_{\mathbf{k}}^{(0)})\rho_{\mathbf{k}}(1 - \rho_{\mathbf{k}}^{(0)}) - \rho_{\mathbf{k}}^{(0)}\rho_{\mathbf{k}}\rho_{\mathbf{k}}^{(0)}$ , this equation can be presented as

$$\rho_{\mathbf{k}D} - \rho_{\mathbf{k}}^{(0)} = (\rho_{\mathbf{k}} - \rho_{\mathbf{k}}^{(0)})(\rho_{\mathbf{k}} - \rho_{\mathbf{k}}^{(0)}) + \frac{i}{2c} \mathbf{B} \cdot \partial_{\mathbf{k}} \rho_{\mathbf{k}} \times \partial_{\mathbf{k}} \rho_{\mathbf{k}}. \quad (7)$$

Note that  $\partial_{\mathbf{k}} \rho_{\mathbf{k}}$  is a matrix and a matrix cross product with itself can be non-zero.

## 2.2. First-order derivatives of the density matrix

To get the first-order derivatives  $\rho_{\mathbf{k}}^{(\mathbf{E})} = \partial \rho_{\mathbf{k}} / \partial \mathbf{E}$  of the density matrix with respect to the electric field of frequency  $\Omega_0$  ( $\mathbf{E} = \mathbf{E}_0 \exp(i\Omega_0 t)$ ), we consider Eq. (6) with  $\Omega = \Omega_0 + i\delta$  (Refs. 1, 4, and 5). The right-hand side in this case is given by

$$\mathcal{R}^{(\mathbf{E})}[\rho_{\mathbf{k}}, n^{(\mathbf{E})}] = -i\partial_{\mathbf{k}} \rho_{\mathbf{k}} - U_{\text{Hxc}}^{(1)}[n^{(\mathbf{E})}]\rho_{\mathbf{k}} \quad (8)$$

with  $\rho_{\mathbf{k}} = \rho_{\mathbf{k}}^{(0)}$ . The diagonal elements of  $\rho_{\mathbf{k}}^{(\mathbf{E})}$  within the occupied and unoccupied subspaces are zero:  $\rho_{\mathbf{k}D}^{(\mathbf{E})} = 0$ .

For the derivative  $\rho_{\mathbf{k}}^{(\mathbf{B})} = \partial \rho_{\mathbf{k}} / \partial \mathbf{B}$  of the density matrix with respect to the static magnetic field,  $\Omega = i\delta$  and the right-hand side is

$$\mathcal{R}^{(\mathbf{B})}[\rho_{\mathbf{k}}, n^{(\mathbf{B})}] = -\frac{i}{2c} (\partial_{\mathbf{k}} \rho_{\mathbf{k}} \times \mathbf{V}_{\mathbf{k}} - \mathbf{V}_{\mathbf{k}} \times \partial_{\mathbf{k}} \rho_{\mathbf{k}}) - U_{\text{Hxc}}^{(1)}[n^{(\mathbf{B})}]\rho_{\mathbf{k}}. \quad (9)$$

As mentioned above,  $n^{(\mathbf{B})} = 0$  for systems with time-reversal symmetry in the ground state.

As follows from Eq. (7), the diagonal elements of  $\rho_{\mathbf{k}}^{(\mathbf{B})}$  within the occupied and unoccupied subspaces are given by

$$\rho_{\mathbf{k}D}^{(\mathbf{B})} = -\frac{i}{2c} \partial_{\mathbf{k}} \rho_{\mathbf{k}}^{(0)} \times \partial_{\mathbf{k}} \rho_{\mathbf{k}}^{(0)}. \quad (10)$$

The derivative  $\rho_{\mathbf{k}}^{(\mathbf{k})} = \partial_{\mathbf{k}} \rho_{\mathbf{k}}^{(0)}$  of the density matrix with respect to the wave vector is calculated within the  $\mathbf{k} \cdot \mathbf{p}$  theory (Ref. 1) considering the perturbation  $P = \mathbf{k}$  and solving Eq. (6) for  $\Omega = 0$  and the right-hand side

$$\mathcal{R}^{(\mathbf{k})}[\rho_{\mathbf{k}}] = -[\mathbf{V}_{\mathbf{k}}, \rho_{\mathbf{k}}] \quad (11)$$

with the diagonal elements equal to zero:  $\rho_{\mathbf{k}D}^{(\mathbf{k})} = 0$ . Clearly  $n^{(\mathbf{k})} = \int_{\text{BZ}} (2\pi)^{-3} d\mathbf{k} \partial_{\mathbf{k}} \rho_{\mathbf{k}}^{(0)} = 0$ .

## 2.3. Second-order derivatives of the density matrix

Let us now discuss the second-order response within the Sternheimer approach<sup>1,6,7</sup>. The second-order derivative  $\rho_{\mathbf{k}}^{(\mathbf{EB})} = \partial^2 \rho_{\mathbf{k}}^{(0)} / \partial \mathbf{E} \partial \mathbf{B}$  of the density matrix with respect to the magnetic and electric fields can be found based on Eq. (6) with  $\Omega = \Omega_0 + i\delta$  and the right-hand side

$$\begin{aligned} \mathcal{R}^{(\mathbf{EB})}[\rho_{\mathbf{k}}^{(\mathbf{E})}, \rho_{\mathbf{k}}^{(\mathbf{B})}, n^{(\mathbf{E})}, n^{(\mathbf{B})}, n^{(\mathbf{EB})}] \\ = \mathcal{R}^{(\mathbf{E})}[\rho_{\mathbf{k}}^{(\mathbf{B})}, n^{(\mathbf{E})}] + \mathcal{R}^{(\mathbf{B})}[\rho_{\mathbf{k}}^{(\mathbf{E})}, n^{(\mathbf{B})}] \\ - \left( 2U_{\text{xc}}^{(2)}[n^{(\mathbf{E})}, n^{(\mathbf{B})}] + U_{\text{Hxc}}^{(1)}[n^{(\mathbf{EB})}] \right) \rho_{\mathbf{k}}^{(0)}. \end{aligned} \quad (12)$$

However, in this case, there is actually no need to solve Eq. (6) explicitly. Instead a supplementary perturbation corresponding to a vector potential  $P = \mathbf{A}$  at frequency  $-\Omega$  with the right-hand side

$$\mathcal{R}^{(\mathbf{A})}[\rho_{\mathbf{k}}, n^{(\mathbf{A})}] = -\frac{1}{c} [\mathbf{V}_{\mathbf{k}}, \rho_{\mathbf{k}}] - U_{\text{Hxc}}^{(1)}[n^{(\mathbf{A})}]\rho_{\mathbf{k}} \quad (13)$$

can be considered.

Let us show that the first-order derivatives with respect to the perturbations  $P = \mathbf{E}, \mathbf{B}$  and  $\mathbf{A}$  are sufficient for calculation of the contribution  $\alpha_{\nu\mu,\gamma}$  to the polarizability in the presence of the magnetic field given by Eq. (20) of the paper. Based on definition of  $\mathcal{R}^{(\mathbf{A})} = R_{\mathbf{k}}^{(\mathbf{A})}$  given by Eq. (13), we can write that

$$\begin{aligned} -\frac{1}{c} \text{Tr} [\mathbf{V} \tilde{\rho}^{(\mathbf{EB})}] = \text{Tr} [R^{(\mathbf{A})}[\rho^{(0)}, n^{(\mathbf{A})}] \tilde{\rho}^{(\mathbf{EB})}] \\ + \int U_{\text{Hxc}}^{(1)}[n^{(\mathbf{A})}] n^{(\mathbf{EB})} d\mathbf{r}. \end{aligned} \quad (14)$$

The terms with  $\tilde{\rho}_{\text{CC}}^{(\mathbf{EB})}$  and  $\tilde{\rho}_{\text{VV}}^{(\mathbf{EB})}$  are determined by the block diagonal part  $\rho_{\mathbf{k}D}^{(\mathbf{EB})}$ , which is expressed through the first-order responses to the magnetic and electric fields (see Eq. (7)) as

$$\begin{aligned} \rho_{\mathbf{k}D}^{(\mathbf{EB})} = \rho_{\mathbf{k}}^{(\mathbf{E})} \rho_{\mathbf{k}}^{(\mathbf{B})} + \rho_{\mathbf{k}}^{(\mathbf{B})} \rho_{\mathbf{k}}^{(\mathbf{E})} \\ - \frac{i}{2c} \mathbf{B} \left( \partial_{\mathbf{k}} \rho_{\mathbf{k}}^{(\mathbf{E})} \times \partial_{\mathbf{k}} \rho_{\mathbf{k}}^{(0)} + \partial_{\mathbf{k}} \rho_{\mathbf{k}}^{(0)} \times \partial_{\mathbf{k}} \rho_{\mathbf{k}}^{(\mathbf{E})} \right). \end{aligned} \quad (15)$$

Then it can be noticed that

$$\begin{aligned} \text{Tr} [R^{(\mathbf{A})} \tilde{\rho}_{\text{CV}}^{(\mathbf{EB})}(\Omega)] \\ = \int_{\text{BZ}} \frac{d\mathbf{k}}{(2\pi)^3} \sum_v \langle \psi_{v\mathbf{k}}^{(0)} | R^{(\mathbf{A})} L_{v\mathbf{k}}^{-1}(\Omega) P_c R^{(\mathbf{EB})} | \psi_{v\mathbf{k}}^{(0)} \rangle \\ = \text{Tr} [\tilde{\rho}_{\text{VC}}^{(\mathbf{A})}(-\Omega) R^{(\mathbf{EB})}], \end{aligned} \quad (16)$$

where the sum is over valence bands  $v$ .

The last term in Eq. (14) can be also represented as

$$\begin{aligned} \int U_{\text{Hxc}}^{(1)}[n^{(\mathbf{A})}] n^{(\mathbf{EB})} d\mathbf{r} \\ = \int f_{\text{Hxc}}(\mathbf{r}, \mathbf{r}') n^{(\mathbf{A})}(\mathbf{r}') n^{(\mathbf{EB})}(\mathbf{r}) d\mathbf{r}' d\mathbf{r} \\ = \text{Tr} [U_{\text{Hxc}}^{(1)}[n^{(\mathbf{EB})}] (\tilde{\rho}_{\text{CV}}^{(\mathbf{A})} + \tilde{\rho}_{\text{VC}}^{(\mathbf{A})})] \end{aligned} \quad (17)$$

Using Eqs. (12), (16) and (17), we finally get

$$\begin{aligned}
& \text{Tr} \left[ R^{(\mathbf{A})} [\rho^{(0)}, n^{(\mathbf{A})}] \left( \tilde{\rho}_{\text{CV}}^{(\mathbf{EB})} + \tilde{\rho}_{\text{VC}}^{(\mathbf{EB})} \right) \right] \\
& + \int U_{\text{Hxc}}^{(1)} [n^{(\mathbf{A})}] n^{(\mathbf{EB})} d\mathbf{r} \\
& = \text{Tr} \left[ \left( \tilde{\rho}_{\text{VC}}^{(\mathbf{A})} + \tilde{\rho}_{\text{CV}}^{(\mathbf{A})} \right) R^{(\mathbf{E})} [\tilde{\rho}^{(\mathbf{B})}, n^{(\mathbf{E})}] \right] \\
& + \text{Tr} \left[ \left( \tilde{\rho}_{\text{VC}}^{(\mathbf{A})} + \tilde{\rho}_{\text{CV}}^{(\mathbf{A})} \right) R^{(\mathbf{B})} [\tilde{\rho}^{(\mathbf{E})}, n^{(\mathbf{B})}] \right] \\
& - 2 \int U_{\text{xc}}^{(2)} [n^{(\mathbf{E})}, n^{(\mathbf{B})}] n^{(\mathbf{A})} d\mathbf{r}.
\end{aligned} \tag{18}$$

Therefore, the contribution  $\alpha_{\nu\mu,\gamma}$  to the polarizability in the presence of the magnetic field can be expressed through the first-order derivatives to the perturbations  $P = \mathbf{E}, \mathbf{B}$  and  $\mathbf{A}$  in accordance with the “ $2n + 1$ ” theorem<sup>6,7</sup>.

Physically there is no difference between the uniform vector potential  $\mathbf{A}$  at frequency  $-\Omega$  and electric field  $\mathbf{E} = -c^{-1}\partial_t\mathbf{A} = i\Omega\mathbf{A}/c$  at the same frequency. Therefore, the observables corresponding to the responses of the electron density are related as  $n^{(\mathbf{A})}(-\Omega) = i\Omega n^{(\mathbf{E})}(-\Omega)/c$ . To find the relation for the projections of the derivatives of the density matrix onto the unperturbed wavefunctions, we use that without account of local-field effects,  $R^{(\mathbf{A})} = c^{-1}R^{(\mathbf{k})}$ , as seen from Eqs. (11) and (13), Eq. (8) for  $R^{(\mathbf{E})}$  and that  $n^{(\mathbf{k})} = 0$ , as discussed before:

$$\begin{aligned}
& c|\eta_{v\mathbf{k}}^{(\mathbf{A})}(-\Omega)\rangle - |\eta_{v\mathbf{k}}^{(\mathbf{k})}\rangle \\
& = (L_{v\mathbf{k}}^{-1}(-\Omega) - L_{v\mathbf{k}}^{-1}(0))P_c R^{(\mathbf{k})}|\psi_{v\mathbf{k}}^{(0)}\rangle \\
& \quad - cL_{v\mathbf{k}}^{-1}(-\Omega)P_c U_{\text{Hxc}}^{(1)}[n^{(\mathbf{A})}(-\Omega)]|\psi_{v\mathbf{k}}^{(0)}\rangle \\
& = \Omega L_{v\mathbf{k}}^{-1}(-\Omega)L_{v\mathbf{k}}^{-1}(0)P_c R^{(\mathbf{k})}|\psi_{v\mathbf{k}}^{(0)}\rangle \\
& \quad - i\Omega L_{v\mathbf{k}}^{-1}(-\Omega)P_c U_{\text{Hxc}}^{(1)}[n^{(\mathbf{E})}(-\Omega)]|\psi_{v\mathbf{k}}^{(0)}\rangle \\
& = \Omega L_{v\mathbf{k}}^{-1}(-\Omega)|\eta_{v\mathbf{k}}^{(\mathbf{k})}\rangle \\
& \quad - i\Omega L_{v\mathbf{k}}^{-1}(-\Omega)P_c U_{\text{Hxc}}^{(1)}[n^{(\mathbf{E})}]|\psi_{v\mathbf{k}}^{(0)}\rangle \\
& = i\Omega L_{v\mathbf{k}}^{-1}(-\Omega)P_c R^{(\mathbf{E})}|\psi_{v\mathbf{k}}^{(0)}\rangle = i\Omega|\eta_{v\mathbf{k}}^{(\mathbf{E})}(-\Omega)\rangle
\end{aligned} \tag{19}$$

Thus, finding the first-order derivative of the density matrix with respect to the supplementary perturbation  $P = \mathbf{A}$  is reduced to the calculations for the electric field at frequency  $-\Omega = -\Omega_0 - i\delta$ . For molecules in a large simulation box, the wavefunctions can be chosen real and then  $|\eta_{v\mathbf{k}}^{(\mathbf{E})}(-\Omega)\rangle = (|\eta_{v\mathbf{k}}^{(\mathbf{E})}(-\Omega^*)\rangle)^*$ . The responses at frequencies  $\Omega$  and  $-\Omega^*$  are computed for the polarizability in the absence of the magnetic field (see Eq. (26) below) and, therefore, no additional calculations for the supplementary perturbation are required in this case.

The second-order derivative  $\rho_{\mathbf{k}}^{(\mathbf{kE})} = \partial_{\mathbf{k}}\rho_{\mathbf{k}}^{(\mathbf{E})}$  of the density matrix with respect to the electric field and wave vector are found from the solution of Eq. (6) at frequency  $\Omega = \Omega_0 + i\delta$  with

$$\begin{aligned}
\mathcal{R}^{(\mathbf{kE})}[\rho_{\mathbf{k}}^{(\mathbf{k})}, \rho_{\mathbf{k}}^{(\mathbf{E})}, n^{(\mathbf{E})}] &= \mathcal{R}^{(\mathbf{E})}[\rho_{\mathbf{k}}^{(\mathbf{k})}, n^{(\mathbf{E})}] \\
&+ \mathcal{R}^{(\mathbf{k})}[\rho_{\mathbf{k}}^{(\mathbf{E})}]
\end{aligned} \tag{20}$$

and  $\rho_{\mathbf{kD}}^{(\mathbf{kE})} = \rho_{\mathbf{k}}^{(\mathbf{k})}\rho_{\mathbf{k}}^{(\mathbf{E})} + \rho_{\mathbf{k}}^{(\mathbf{E})}\rho_{\mathbf{k}}^{(\mathbf{k})}$ .

For the second-order derivative  $\rho_{\mathbf{k}}^{(\mathbf{kB})} = \partial_{\mathbf{k}}\rho_{\mathbf{k}}^{(\mathbf{B})}$  of the density matrix with respect to the static magnetic field and wave vector, we use  $\Omega = i\delta$ ,

$$\begin{aligned}
\mathcal{R}^{(\mathbf{kB})}[\rho_{\mathbf{k}}^{(\mathbf{k})}, \tilde{\rho}_{\mathbf{k}}^{(\mathbf{B})}, \tilde{\rho}_{\mathbf{k}}^{(0)}, n^{(\mathbf{B})}] &= \mathcal{R}^{(\mathbf{B})}[\rho_{\mathbf{k}}^{(\mathbf{k})}, n^{(\mathbf{B})}] \\
&+ \mathcal{R}^{(\mathbf{k})}[\rho_{\mathbf{k}}^{(\mathbf{B})}] + \mathcal{R}^{(\mathbf{kB},2)}[\rho_{\mathbf{k}}^{(0)}],
\end{aligned} \tag{21}$$

where

$$\mathcal{R}^{(\mathbf{kB},2)}[\rho_{\mathbf{k}}] = \frac{e_{\alpha\beta\gamma}}{2c} \left( [r_{\mu}, V_{\mathbf{k}\beta}] \frac{\partial \rho_{\mathbf{k}}}{\partial k_{\gamma}} - \frac{\partial \rho_{\mathbf{k}}}{\partial k_{\beta}} [r_{\mu}, V_{\mathbf{k}\gamma}] \right), \tag{22}$$

and

$$\begin{aligned}
\rho_{\mathbf{kD}}^{(\mathbf{kB})} &= \rho_{\mathbf{k}}^{(\mathbf{k})}\rho_{\mathbf{k}}^{(\mathbf{B})} + \rho_{\mathbf{k}}^{(\mathbf{B})}\rho_{\mathbf{k}}^{(\mathbf{k})} \\
&- \frac{i}{2c} \left( \partial_{\mathbf{k}}\rho_{\mathbf{k}}^{(\mathbf{k})} \times \partial_{\mathbf{k}}\rho_{\mathbf{k}}^{(0)} + \partial_{\mathbf{k}}\rho_{\mathbf{k}}^{(0)} \times \partial_{\mathbf{k}}\rho_{\mathbf{k}}^{(\mathbf{k})} \right).
\end{aligned} \tag{23}$$

The second-order derivative  $\rho_{\mathbf{k}}^{(\mathbf{kB})} = \partial_{\mathbf{k}}\rho_{\mathbf{k}}^{(\mathbf{k})}$  of the density matrix with respect to the wave vector is calculated using Eq. (6) for  $\Omega = 0$  and

$$\mathcal{R}^{(\mathbf{kB})}[\rho_{\mathbf{k}}^{(\mathbf{k})}, \rho_{\mathbf{k}}^{(0)}] = \mathcal{R}^{(\mathbf{k})}[\rho_{\mathbf{k}}^{(\mathbf{k})}] + \mathcal{R}^{(2,\mathbf{kB})}[\rho_{\mathbf{k}}^{(0)}], \tag{24}$$

where

$$\mathcal{R}^{(2,\mathbf{kB})}[\rho_{\mathbf{k}}] = \frac{i}{2} [[r_{\alpha}, V_{\mathbf{k}\beta}], \rho_{\mathbf{k}}]. \tag{25}$$

The corresponding diagonal elements are determined by  $\rho_{\mathbf{kD}}^{(\mathbf{kB})} = \rho_{\mathbf{k}}^{(\mathbf{k})}\rho_{\mathbf{k}}^{(\mathbf{k})}$ .

Similar to  $n^{(\mathbf{k})}$ ,  $n^{(\mathbf{kE})} = 0$ ,  $n^{(\mathbf{kB})} = 0$  and  $n^{(\mathbf{kB})} = 0$ .

#### 2.4. Polarizability in the absence of the magnetic field

The polarizability in the absence of the magnetic field is given by Eq. (19) of the paper. Using Eq. (19) from the previous subsection, this expression can be written as

$$\begin{aligned}
\alpha_{0\nu\mu}(\Omega) &= \frac{1}{\Omega} \int_{\text{BZ}} \frac{d\mathbf{k}}{(2\pi)^3} \sum_v \left( \langle \eta_{v\mathbf{k}}^{(k_{\mu})} | \eta_{v\mathbf{k}}^{(k_{\nu})} \rangle \right. \\
&\quad \left. - \langle \eta_{v\mathbf{k}}^{(k_{\nu})} | \eta_{v\mathbf{k}}^{(k_{\mu})} \rangle \right. \\
&\quad \left. + i\Omega \langle \eta_{v\mathbf{k}}^{(k_{\nu})} | \eta_{v\mathbf{k}}^{(E_{\mu})}(\Omega) \rangle - i\Omega \langle \eta_{v\mathbf{k}}^{(E_{\mu})}(-\Omega^*) | \eta_{v\mathbf{k}}^{(k_{\nu})} \rangle \right),
\end{aligned} \tag{26}$$

where the sum is over valence bands  $v$ . If the Berry curvature in the first two lines of this expression is zero (like for the systems considered in the present paper), the polarizability takes the same form as in Refs. 1 and 5.

## 2.5. Band magnetic dipole moments

The orbital magnetic dipole moments of bands<sup>8,9</sup> are computed as

$$m_{\gamma,n\mathbf{k}} = i \frac{e_{\alpha\beta\gamma}}{2c} \sum_p \frac{\langle \psi_{n\mathbf{k}}^{(0)} | V_{\alpha} | \psi_{p\mathbf{k}}^{(0)} \rangle \langle \psi_{p\mathbf{k}}^{(0)} | V_{\beta} | \psi_{n\mathbf{k}}^{(0)} \rangle}{\epsilon_{p\mathbf{k}} - \epsilon_{n\mathbf{k}}}, \quad (27)$$

where the sum is taken over all bands  $p$  which are non-degenerate with the band  $n$  at  $\mathbf{k}$ -point  $\mathbf{k}$ .

Using 60 unoccupied bands for silicon, the magnetic dipole moments of the highest occupied  $\Gamma'_{25}$  and lowest unoccupied  $\Gamma_{15}$  states with the orbital angular momenta  $l_z = \pm 1$  at the  $\Gamma$  point of the Brillouin zone are found to be  $\pm 0.37\mu_B$  and  $\pm 3.5\mu_B$ , respectively. Using 40 unoccupied bands for boron nitride, the magnetic dipole moments of the highest occupied and lowest unoccupied states at the  $K^{\pm}$  points of the Brillouin zone are calculated to be  $\mp 0.95\mu_B$  and  $\mp 2.8\mu_B$ , respectively.

For valence bands  $v$ , almost same results can be obtained using

$$m_{\gamma,v\mathbf{k}} = i \frac{e_{\alpha\beta\gamma}}{2c} \langle \eta_{v\mathbf{k}}^{(k_{\alpha})} | H_0 - \epsilon_{v\mathbf{k}} | \eta_{v\mathbf{k}}^{(k_{\beta})} \rangle, \quad (28)$$

where no conduction bands are needed. In this way, we compute the magnetic moments of  $\Gamma'_{25}$  states in silicon to be  $\pm 0.40\mu_B$ . For the highest occupied states of boron nitride at the  $K^{\pm}$  points, we find  $\mp 0.95\mu_B$ .

## 3. FINITE-SYSTEM FORMULATION

### 3.1. Equations solved

For finite systems, the Liouville equation for the density matrix can be straightforwardly written in the Coulomb gauge as

$$\Omega\rho + [H, \rho] = [\mathbf{d} \cdot \mathbf{E} + \mathbf{m} \cdot \mathbf{B}, \rho], \quad (29)$$

where  $\mathbf{d} = -\mathbf{r}$  is the electric dipole moment and  $\mathbf{m} = -\mathbf{r} \times \mathbf{V}/2c$  is the orbital magnetic dipole moment.

The first-order derivatives  $\rho^{(\mathbf{E})}$  and  $\rho^{(\mathbf{B})}$  are then computed using  $\rho_D^{(\mathbf{E})} = \rho_D^{(\mathbf{B})} = 0$ , right-hand sides

$$R^{(\mathbf{E})}[\rho] = (\mathbf{d} - U_{\text{Hxc}}^{(1)}[n^{(\mathbf{E})}])\rho \quad (30)$$

and

$$R^{(\mathbf{B})}[\rho] = (\mathbf{m} - U_{\text{Hxc}}^{(1)}[n^{(\mathbf{B})}])\rho, \quad (31)$$

and frequencies  $\Omega = \Omega_0 + i\delta$  and  $\Omega = i\delta$ , respectively.

The polarizability  $\alpha_{0\nu\mu}$  in the absence of the magnetic field and the change in the polarizability  $\alpha_{\nu\mu,\gamma}B_{\gamma}$  in the presence of the magnetic field for finite systems can be calculated directly as

$$\alpha_{0\nu\mu}(\Omega) = \text{Tr} [d_{\nu}\rho^{(E_{\mu})}(\Omega)], \quad (32)$$

and

$$\alpha_{\nu\mu,\gamma}(\Omega) = \text{Tr} [d_{\nu}\rho^{(E_{\mu}B_{\gamma})}(\Omega)], \quad (33)$$

respectively.

Making the use of the “ $2n + 1$ ” theorem<sup>6,7</sup>, explicit calculation of the second-order derivative  $\rho^{(\mathbf{EB})}$  can be avoided. Instead a supplementary perturbation  $\mathbf{A}$ , which in this case corresponds to the electric field at frequency  $-\Omega$ , can be introduced:

$$\begin{aligned} \text{Tr} [\mathbf{d}\rho^{(\mathbf{EB})}(\Omega)] &= \text{Tr} [R^{(\mathbf{A})}\rho^{(\mathbf{EB})}(\Omega)] \\ &+ \int U_{\text{Hxc}}^{(1)}[n^{(\mathbf{A})}]n^{(\mathbf{EB})}\mathbf{dr}. \end{aligned} \quad (34)$$

Then the terms with  $\rho_{\text{CC}}^{(\mathbf{EB})}$  and  $\rho_{\text{VV}}^{(\mathbf{EB})}$  (Eq. (14) of the paper) can be determined from the idempotency condition  $\rho_{\text{D}}^{(\mathbf{EB})} = \rho^{(\mathbf{E})}\rho^{(\mathbf{B})} + \rho^{(\mathbf{B})}\rho^{(\mathbf{E})}$ . The terms with  $\rho_{\text{CV}}^{(\mathbf{EB})}$ ,  $\rho_{\text{VC}}^{(\mathbf{EB})}$  and  $n^{(\mathbf{EB})}$  can be written in the way analogous to Eq. (18). In the case of real wavefunctions,  $|\eta_v^{(\mathbf{A})}(-\Omega)\rangle = (|\eta_v^{(\mathbf{E})}(-\Omega^*)\rangle)^*$  and there is no need to solve additionally the Liouville equation for the supplementary perturbation.

### 3.2. $\mathcal{A}$ and $\mathcal{B}$ terms

The polarizability of finite systems

$$\alpha_{\nu\mu}(\Omega) = \tilde{\alpha}_{\nu\mu}(\Omega) + \tilde{\alpha}_{\nu\mu}(-\Omega), \quad (35)$$

can be expressed through sums over molecular states as

$$\tilde{\alpha}_{\nu\mu}(\Omega) = \sum_n \frac{\langle 0|d_{\nu}|n\rangle\langle n|d_{\mu}|0\rangle}{\Omega_n - \Omega}, \quad (36)$$

where  $\Omega_n$  is the transition frequency for the excited state  $n$ .

In the presence of the magnetic field, the molecular states are perturbed and the corresponding contribution to the polarizability gives rise to the  $\mathcal{B}$  term<sup>10-12</sup>

$$\begin{aligned} \tilde{\alpha}_{\nu\mu,\gamma}^{\mathcal{B}}(\Omega) &= \sum_{n \neq p} \frac{\langle 0|d_{\nu}|n\rangle\langle n|m_{\gamma}|p\rangle\langle p|d_{\mu}|0\rangle}{(\Omega_n - \Omega)(\Omega_p - \Omega)} \\ &+ \sum_{n,p} \left\{ \frac{\langle 0|d_{\nu}|n\rangle\langle n|\bar{d}_{\mu}|p\rangle\langle p|m_{\gamma}|0\rangle}{(\Omega_n - \Omega)\Omega_p} \right. \\ &\left. + \frac{\langle 0|m_{\gamma}|n\rangle\langle n|\bar{d}_{\nu}|p\rangle\langle p|d_{\mu}|0\rangle}{\Omega_n(\Omega_p - \Omega)} \right\}, \end{aligned} \quad (37)$$

where the overline denotes the fluctuation operators  $\bar{O} = O - \langle 0|O|0\rangle$ . It is clear from this equation that the  $\mathcal{B}$  term introduces only first-order poles and the height of the corresponding peaks is inversely proportional to the linewidth.

The magnetic field, however, also affects the energies of the molecular states. Such a contribution is referred to as the  $\mathcal{A}$  term and is given by<sup>10,11,13</sup>

$$\tilde{\alpha}_{\nu\mu,\gamma}^{\mathcal{A}}(\Omega) = \sum_n \frac{\langle 0|d_\nu|n\rangle\langle n|\tilde{m}_\gamma|n\rangle\langle n|d_\mu|0\rangle}{(\Omega_n - \Omega)(\Omega_n - \Omega)}. \quad (38)$$

This term describing the linear response to the magnetic field is sufficient as long as  $|\langle n|\tilde{m}_\gamma|n\rangle B_\gamma| \ll |\Omega_n - \Omega|$ . At resonances, this means that the Zeeman splitting should be smaller than the linewidth. Using the typical linewidth  $\delta \sim 0.1$  eV and magnetic moment change on the order of the Bohr magneton  $\mu_B$ , one finds that the expression is valid even for rather strong magnetic fields  $B \ll \delta/\mu_B \sim 10^3$  T.

As seen from Eqs. (36) and (38), close to the resonances, the  $\mathcal{A}$  term is determined by the derivative of the spectral function weighted by the magnetic moment change upon the excitation. Correspondingly it is present only for molecules with rotational symmetry at least of the third order, which have degenerate states with non-zero orbital momenta, and is manifested through second-order poles in the magneto-optical spectra. The height of the corresponding peaks is inversely proportional to the linewidth squared.

It also follows from Eqs. (36) and (38) that the ratio of the  $\mathcal{A}$  term and polarizability in the absence of the magnetic field at the resonance frequency characterizes the change in the orbital magnetic moment  $\Delta\mathbf{m}$  upon the excitation. As discussed above, the  $\mathcal{A}$  term is non-zero only for symmetric systems, where there is an axis of rotational symmetry at least of the third order (let us denote it  $z$ ). For such systems,  $|\langle 0|d_x|n\rangle| = |\langle 0|d_y|n\rangle|$ . Using that  $\Omega_n - \Omega = -i\delta$  and the selection rule for the magnetic quantum number  $\Delta l_z = \pm 1$ , one gets

$$\tilde{\alpha}_{xy,z}^{\mathcal{A}}/\tilde{\alpha}_{xx} \sim \Delta m_z \Delta l_z / \delta \quad (39)$$

#### 4. ANGLE OF FARADAY ROTATION AND ELLIPTICITY

Let us establish the relationships between the non-diagonal elements of the electric susceptibility tensor  $\chi_{\nu\mu} = \alpha_{\nu\mu}/w$ , where  $w$  is the unit cell volume, and the angle of rotation  $\phi_z$  and ellipticity  $\theta_z$  gained by the linearly polarized light when it passes through the crystal<sup>14</sup>. It should be noted that these relationships are the same in the cases of the magnetic field applied and natural optical activity.

We consider a plane wave propagating through the crystal along the axis  $z$ ,

$$\begin{aligned} \tilde{\mathbf{E}} &= \tilde{\mathbf{E}}_0 e^{i(n\Omega z/c + \Omega t)}, \\ \tilde{\mathbf{B}} &= \tilde{\mathbf{B}}_0 e^{i(n\Omega z/c + \Omega t)}, \end{aligned} \quad (40)$$

where  $n$  is the refractive index. We assume that the axis  $z$  is the optical axis so that no birefringence takes place.

In the absence of external charges and currents, the Maxwell equations can be written as

$$\begin{aligned} \nabla \times \tilde{\mathbf{E}} &= -\frac{1}{c} \frac{\partial \tilde{\mathbf{B}}}{\partial t}, & \nabla \times \tilde{\mathbf{H}} &= \frac{1}{c} \frac{\partial \tilde{\mathbf{D}}}{\partial t}, \\ \nabla \cdot \tilde{\mathbf{D}} &= 0, & \nabla \cdot \tilde{\mathbf{B}} &= 0, \end{aligned} \quad (41)$$

where  $\mathbf{D}$  is the displacement field and  $\mathbf{H}$  is the magnetizing field. Assuming  $\mathbf{B} \approx \mathbf{H}$  one gets

$$\nabla \times \nabla \times \tilde{\mathbf{E}} = \left(\frac{\Omega}{c}\right)^2 \tilde{\mathbf{D}}, \quad \nabla \cdot \tilde{\mathbf{D}} = 0. \quad (42)$$

In the absence of the magnetic field or natural optical activity,  $\chi_{0xx} = \chi_{0yy} = (n_0^2 - 1)/4\pi$ , where  $n_0$  is the ordinary refractive index, and  $\chi_{0\mu\nu} = 0$  for any  $\mu \neq \nu$ . In the presence of the magnetic field or natural optical activity, we assume that  $\chi_{xx} \approx \chi_{yy}$  and  $\chi_{xy} = -\chi_{yx}$  are much smaller in magnitude than  $\chi_{0xx}$ . Using that  $\tilde{D}_\mu = \tilde{E}_\mu + 4\pi\tilde{P}_\mu = (\delta_{\mu\nu} + 4\pi\chi_{\mu\nu})\tilde{E}_\nu$ , where  $\tilde{P}$  is the bulk polarization, the first of Eq. (42) is reduced to

$$\begin{pmatrix} n^2 - 1 - 4\pi\chi_{xx} & -4\pi\chi_{xy} \\ -4\pi\chi_{yx} & n^2 - 1 - 4\pi\chi_{yy} \end{pmatrix} \begin{pmatrix} E_x \\ E_y \end{pmatrix} = 0 \quad (43)$$

and gives  $n^\pm - n_0 \approx \pm 2\pi i\chi_{xy}/n_0$ . The two solutions correspond to the left (+) and right (−) circularly polarized light with  $E_y = \pm iE_x$ .

The angle of rotation  $\phi_z$  and ellipticity  $\theta_z$  gained at distance  $l$  are expressed through the real and imaginary parts of refractive indices  $n^\pm$  as (Ref. 14)

$$\begin{aligned} \phi_z(\Omega_0) &= \frac{\Omega_0 l}{2c} \text{Re}(n^+ - n^-), \\ \theta_z(\Omega_0) &= \frac{\Omega_0 l}{2c} \text{Im}(n^+ - n^-), \end{aligned} \quad (44)$$

which gives

$$\begin{aligned} \phi_z(\Omega_0) &= -\frac{\pi\Omega_0 l}{c} \text{Im} \left[ \frac{\chi_{xy}(\Omega) - \chi_{yx}(\Omega)}{n_0} \right], \\ \theta_z(\Omega_0) &= \frac{\pi\Omega_0 l}{c} \text{Re} \left[ \frac{\chi_{xy}(\Omega) - \chi_{yx}(\Omega)}{n_0} \right]. \end{aligned} \quad (45)$$

The angle of rotation and ellipticity arising from the effect of the magnetic field and corresponding to the Faraday rotation and MCD signal, respectively, can, therefore, be found as

$$\begin{aligned} \phi_z(\Omega_0) &= -\frac{\pi\Omega_0 l}{c} B_z \text{Im} \left[ \frac{\chi_{xy,z}(\Omega) - \chi_{yx,z}(\Omega)}{n_0} \right], \\ \theta_z(\Omega_0) &= \frac{\pi\Omega_0 l}{c} B_z \text{Re} \left[ \frac{\chi_{xy,z}(\Omega) - \chi_{yx,z}(\Omega)}{n_0} \right]. \end{aligned} \quad (46)$$

It should be emphasized that the assumption of  $z$  being the axis of rotational symmetry is used above only to derive the relationship between the polarizability  $\alpha_{\nu\mu} = w\chi_{\nu\mu}$  and physical properties like ellipticity and angle of rotation, which make sense only when the

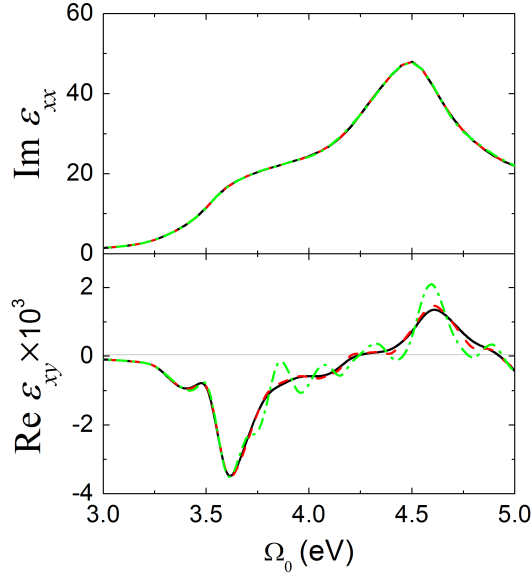

FIG. 1. Calculated components  $\text{Im } \epsilon_{xx}$  (upper panel) and  $\text{Re } \epsilon_{xy}$  (lower panel) of the dielectric tensor of silicon as functions of the frequency of light  $\Omega_0$  (in eV) for the magnetic field of 1 T along the  $z$  axis. The data obtained in the independent particle approximation using 48266 irreducible k-points (shifted  $8 \times 8 \times 8$  k-point grids giving the grid of  $128 \times 128 \times 128$  in total), 6586 irreducible k-points ( $64 \times 64 \times 64$  grid in total) and 1010 irreducible k-points ( $32 \times 32 \times 32$  grid in total) are shown by black solid, red dashed and green dash-dotted lines, respectively. The calculated data are blue-shifted in energy by 0.7 eV to take into account the GW correction to the band gap<sup>15,16</sup>.

light components with right and left circular polarization propagate at almost equal speed. Eq. (20) of the paper for  $\alpha_{\nu\mu,\gamma}$  does not rely on this assumption and can be used to compute the polarizability tensor in the presence of the magnetic field for any arbitrary system, including highly anisotropic ones.

## 5. ADDITIONAL DETAILS AND RESULTS OF CALCULATIONS

### 5.1. k-point grids and local-field effects

A large number of k-points is required to converge the magneto-optical spectra of solids. To achieve the necessary number of k-points, shifted k-point grids are considered. Uniform  $8 \times 8 \times 8$  and  $10 \times 18 \times 1$  grids are used for silicon and boron nitride, respectively. These grids are sufficient to converge well the eigenstates. The shifts of  $m_i \Delta k_i / n_i$  with  $m_i = 0, 1, \dots, n_i - 1$  are applied along the orthogonal axes  $i = 1 - 3$ , where  $\Delta k_i$  corresponds to the spacing of the single grid along the axis  $i$ . In this way, the shifted grids constitute in total the uniform grid with the spacing of  $\Delta k_i / n_i$  along the axis  $i$ . For silicon, the cases of  $n_1 = n_2 = n_3 = 4, 8$  and 16 have been considered

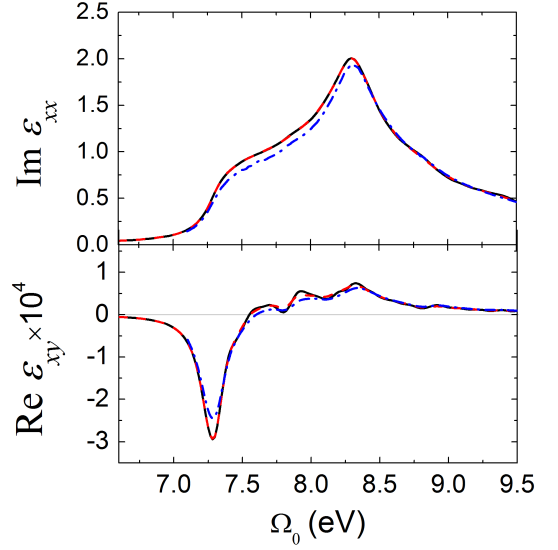

FIG. 2. Calculated components  $\text{Im } \epsilon_{xx}$  (upper panel) and  $\text{Re } \epsilon_{xy}$  (lower panel) of the dielectric tensor of boron nitride monolayer as functions of the frequency of light  $\Omega_0$  (in eV) for the magnetic field of 1 T along the  $z$  axis directed out of the plane.  $x$  and  $y$  axes are aligned along the armchair and zigzag directions. The data obtained in the independent particle approximation using 2993 irreducible k-points (shifted  $10 \times 18 \times 1$  k-point grids giving the grid of  $80 \times 144 \times 1$  in total) and 11745 irreducible k-points ( $160 \times 288 \times 1$  grid in total) are shown by black solid and red dashed lines, respectively. The results calculated with account of the local-field effects in the ALDA approximation using 11745 irreducible k-points are represented by blue dash-dotted lines. The calculated data are blue-shifted in energy by 2.6 eV to take into account the GW correction to the band gap<sup>17</sup>.

(Fig. 1). For boron nitride,  $n_1 = n_2 = 8$  and 16 have been studied (Fig. 2; along the out-of-plane axis  $n_3 = 1$ ).

Figs. 1 and 2 show that at least 6600 and 3000 irreducible k-points are required to converge the MCD spectra for silicon and boron nitride, respectively. Fig. 2 also demonstrates that the account of local-field effects in the adiabatic local-density approximation (ALDA) leads to a small correction of the absorption and MCD spectra for boron nitride.

The influence of the parameter  $\beta$  in Eq. (37) of the paper derived<sup>18</sup> for excitonic effects in the framework of time-dependent current density functional theory (TD-CDFT) on the absorption and magneto-optical spectra of boron nitride is demonstrated in Fig. 3. For  $\beta = 8 - 20$ , the prominent excitonic peak is observed and the shapes of the spectra almost do not change upon changing  $\beta$ . The value  $\beta = 17.5$  corresponds to the position of the peak in accordance with the Bethe-Salpeter calculations<sup>17</sup>.

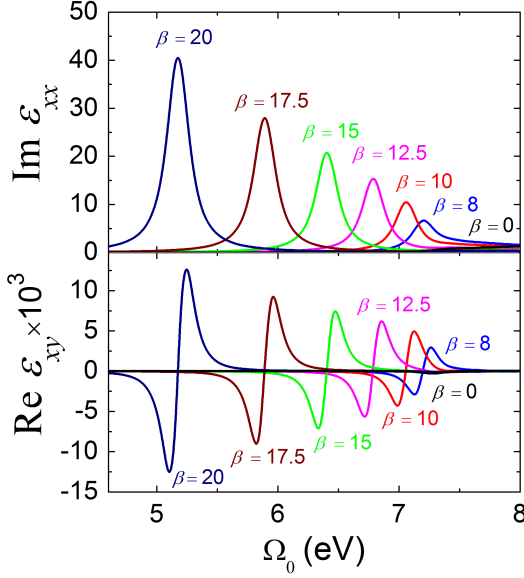

FIG. 3. Components  $\text{Im } \epsilon_{xx}$  (upper panel) and  $\text{Re } \epsilon_{xy}$  (lower panel) of the dielectric tensor of boron nitride monolayer as functions of the frequency of light  $\Omega_0$  (in eV) calculated using different values of the parameter  $\beta$  in Eq. (37) of the paper describing excitonic effects and derived using the TDCDFT polarization functional<sup>18</sup>: (black) 0, (blue) 8, (red) 10, (magenta) 12.5, (green) 15, (brown) 17.5, (dark blue) 20. The magnetic field of 1 T is directed along the  $z$  axis, i.e. out of the plane. The calculated data are blue-shifted in energy by 2.6 eV to take into account the GW correction to the band gap<sup>17</sup>.

### 5.2. Valley g-factor from tight-binding model

According to our estimate, the valley g-factor for the first excitonic peak in boron nitride is about twice smaller than the g-factors measured for excitons in WSe<sub>2</sub> (Refs. 19–21) and MoSe<sub>2</sub> (Refs. 21–23) monolayers. These experimental results are normally interpreted on the basis of the simple two-band tight-binding model<sup>24–26</sup> for the electronic states near the  $K^\pm$  points. It is assumed<sup>19,22,23</sup> that the total magnetic moment of a charge carrier is composed of the intercellular contribution from phase winding of delocalized Bloch wavefunctions at  $K^\pm$  points,  $\mu_k$ , the intracellular contribution of parent atomic orbitals,  $\mu_l$ , and contribution of carrier spin,  $\mu_s$ . In the  $K^+$  valley of WSe<sub>2</sub> and MoSe<sub>2</sub>, these contributions for the conduction ( $c$ ) and valence ( $v$ ) bands are  $\mu_s^c = \mu_s^v = -\mu_B$ ,  $\mu_l^c = 0$ ,  $\mu_l^v = -2\mu_B$ ,  $\mu_k^c = -\mu_B m_0/m_*^c$  and  $\mu_k^v = -\mu_B m_0/m_*^v$ , where  $m_0$  is the free electron mass and  $m_*^c$  and  $m_*^v$  are the effective masses for the conduction and valence bands<sup>23</sup>. For the contribution of atomic orbitals, it is taken into account that the highest valence bands in WSe<sub>2</sub> and MoSe<sub>2</sub> are predominantly composed of  $d_{x^2-y^2} \pm id_{xy}$  W/Mo orbitals with  $l_z = \pm 2$  and the lowest conduction bands of  $d_z^2$  W/Mo orbitals with  $l_z = 0$  (Refs. 27). The coupled spin and valley

physics in group-IV dichalcogenides provides that the spin degree of freedom is frozen out and the spin contributions are the same for the valence and conduction bands<sup>28</sup>. In the model with just two bands, the intercellular contributions to the magnetic dipole moments are the same in the conduction and valence bands<sup>24–26</sup>. As a result, the tight-binding model<sup>24–26</sup> shows that the change of the magnetic dipole moment upon the excitation in WSe<sub>2</sub> and MoSe<sub>2</sub> is mostly related to the contribution of parent atomic orbitals<sup>19,22,23</sup>. Indeed the corresponding valley g-factor of 4 is close to the result of experimental observations<sup>19–23</sup> for WSe<sub>2</sub> and MoSe<sub>2</sub>.

The contribution from parent atomic orbitals is absent in boron nitride, where the first optical transitions take place between the bands composed of  $p_z$  orbitals with  $l_z = 0$  (Ref. 29). Therefore, the tight-binding model<sup>24–26</sup> gives a vanishing g-factor for boron nitride. The valley g-factor for boron nitride is, nevertheless, significant according to our calculations and comparable to the results for WSe<sub>2</sub> and MoSe<sub>2</sub>. Therefore, the model<sup>24–26</sup> is not adequate for description of band magnetic dipole moments in boron nitride. Calculations of band magnetic dipole moments for WSe<sub>2</sub> and MoSe<sub>2</sub> with account of a large number of bands are required to explain properly the g-factors observed for these materials (see also Ref. 21).

### 5.3. Computational time

Let us now discuss the computational time required for calculations of the magneto-optical spectra for solids. The perturbations  $P = \mathbf{B}$ ,  $\mathbf{k}$ ,  $\mathbf{k}\mathbf{k}$  and  $\mathbf{k}\mathbf{B}$  are static and the corresponding derivatives of the density matrix are computed only once at zero frequency. The perturbations  $P = \mathbf{E}$  and  $\mathbf{k}\mathbf{E}$  at frequencies  $\Omega = \pm\Omega_0 + i\delta$  and supplementary perturbation  $\mathbf{A}$ , which is reduced to the perturbation  $P = \mathbf{E}$  at frequencies  $\Omega = \pm\Omega_0 - i\delta$  (see Eqs. (14)–(19) of section 2.3), have to be considered at each frequency  $\Omega_0$ . If time-reversal symmetry is taken into account, the response to the perturbation  $\mathbf{k}\mathbf{E}$  should also be found at frequencies  $\Omega = \pm\Omega_0 - i\delta$ . For the perturbation  $\mathbf{E}$ , Eq. (6) has to be solved three times at each frequency  $\Omega$  for the components of the electric field  $\mathbf{E}$  along three orthogonal axes. For the perturbation  $\mathbf{k}\mathbf{E}$ , the equation has to be solved 9 times for three components of the electric field  $\mathbf{E}$  and three components of the wave vector  $\mathbf{k}$ . Thus, Eq. (6) is solved 12 times at each frequency  $\Omega$ , i.e. 48 times at each frequency  $\Omega_0$  since  $\Omega = \pm\Omega_0 \pm i\delta$ .

In the absence of the magnetic field, only the response to the perturbation  $\mathbf{E}$  at frequencies  $\Omega = \pm\Omega_0 + i\delta$  is needed (see Eq. (26)). Therefore, Eq. (6) is solved 6 times at each frequency  $\Omega_0$ . This means that if the local-field effects are not taken into account in Eq. (6), the calculation of magneto-optical spectra can be up to 8 times slower than of optical polarizability in the absence of the magnetic field given that the calculation parameters

(k-point and real-space grids, etc.) are the same.

If local-field effects are taken into account, the computational time grows considerably because of the steps where Eq. (6) is solved self-consistently. The perturbation  $\mathbf{kE}$  does not lead to changes in the electron density<sup>1</sup> and no self-consistent calculations are required. The speed-limiting step is the calculation of the self-

consistent response to the electric field  $\mathbf{E}$  at frequencies  $\Omega = \pm\Omega_0 \pm i\delta$ . Since the number of frequencies is doubled as compared to the case when the magnetic field is absent ( $\Omega = \pm\Omega_0 + i\delta$ ), the calculation of magneto-optical spectra for solids takes about twice as long as simple optical polarizability.

\* liv.ira@hotmail.com

† angel.rubio@mpsd.mpg.de

<sup>1</sup> D. A. Strubbe, *Optical and transport properties of organic molecules: Methods and applications* (PhD thesis, University of California, Berkeley, USA, 2012).

<sup>2</sup> A. M. Essin, A. M. Turner, J. E. Moore, and D. Vanderbilt, “Orbital magnetoelectric coupling in band insulators,” *Phys. Rev. B* **81**, 205104 (2010).

<sup>3</sup> X. Gonze and J. W. Zwanziger, “Density-operator theory of orbital magnetic susceptibility in periodic insulators,” *Phys. Rev. B* **84**, 064445 (2011).

<sup>4</sup> D. A. Strubbe, L. Lehtovaara, A. Rubio, M. A. L. Marques, and S. G. Louie, “Response functions in TDDFT: Concepts and implementation,” in *Fundamentals of Time-Dependent Density Functional Theory*, edited by M. A. L. Marques, N. T. Maitra, F. M. S. Nogueira, E. K. U. Gross, and A. Rubio (Springer Berlin Heidelberg, Berlin, Heidelberg, 2012) pp. 139–166.

<sup>5</sup> X. Andrade and et al., “Real-space grids and the Octopus code as tools for the development of new simulation approaches for electronic systems,” *Phys. Chem. Chem. Phys.* **17**, 31371–31396 (2015).

<sup>6</sup> X. Gonze and J.-P. Vigneron, “Density-functional approach to nonlinear-response coefficients of solids,” *Phys. Rev. B* **39**, 13120–13128 (1989).

<sup>7</sup> A. Dal Corso, F. Mauri, and A. Rubio, “Density-functional theory of the nonlinear optical susceptibility: Application to cubic semiconductors,” *Phys. Rev. B* **53**, 15638–15642 (1996).

<sup>8</sup> J. Shi, G. Vignale, D. Xiao, and Q. Niu, “Quantum theory of orbital magnetization and its generalization to interacting systems,” *Phys. Rev. Lett.* **99**, 197202 (2007).

<sup>9</sup> M.-C. Chang and Q. Niu, “Berry phase, hyperorbits, and the Hofstadter spectrum: Semiclassical dynamics in magnetic Bloch bands,” *Phys. Rev. B* **53**, 7010–7023 (1996).

<sup>10</sup> H. Solheim, K. Ruud, S. Coriani, and P. Norman, “Complex polarization propagator calculations of magnetic circular dichroism spectra,” *J. Chem. Phys.* **128**, 094103 (2008).

<sup>11</sup> K.-M. Lee, K. Yabana, and G. F. Bertsch, “Magnetic circular dichroism in real-time time-dependent density functional theory,” *J. Chem. Phys.* **134**, 144106 (2011).

<sup>12</sup> M. Seth, M. Krykunov, T. Ziegler, J. Autschbach, and A. Banerjee, “Application of magnetically perturbed time-dependent density functional theory to magnetic circular dichroism: Calculation of B terms,” *J. Chem. Phys.* **128**, 144105 (2008).

<sup>13</sup> M. Seth, M. Krykunov, T. Ziegler, and J. Autschbach, “Application of magnetically perturbed time-dependent density functional theory to magnetic circular dichroism. II. Calculation of A terms,” *J. Chem. Phys.* **128**, 234102

(2008).

<sup>14</sup> L. D. Barron, *Molecular Light Scattering and Optical Activity*, 2nd ed. (Cambridge University Press, Cambridge, 2004).

<sup>15</sup> S. Albrecht, L. Reining, R. Del Sole, and G. Onida, “Ab initio calculation of excitonic effects in the optical spectra of semiconductors,” *Phys. Rev. Lett.* **80**, 4510–4513 (1998).

<sup>16</sup> S. Botti and et al., “Long-range contribution to the exchange-correlation kernel of time-dependent density functional theory,” *Phys. Rev. B* **69**, 155112 (2004).

<sup>17</sup> L. Wirtz, A. Marini, and A. Rubio, “Optical absorption of hexagonal boron nitride and BN nanotubes,” *AIP Conf. Proc.* **786**, 391–395 (2005).

<sup>18</sup> J. A. Berger, “Fully parameter-free calculation of optical spectra for insulators, semiconductors, and metals from a simple polarization functional,” *Phys. Rev. Lett.* **115**, 137402 (2015).

<sup>19</sup> A. Srivastava and et al., “Valley Zeeman effect in elementary optical excitations of monolayer WSe<sub>2</sub>,” *Nat. Phys.* **11**, 141–147 (2015).

<sup>20</sup> A. A. Mitroglu and et al., “Optical investigation of monolayer and bulk tungsten diselenide (WSe<sub>2</sub>) in high magnetic fields,” *Nano Lett.* **15**, 4387–4392 (2015).

<sup>21</sup> G. Wang and et al., “Magneto-optics in transition metal diselenide monolayers,” *2D Materials* **2**, 034002 (2015).

<sup>22</sup> D. MacNeill and et al., “Breaking of valley degeneracy by magnetic field in monolayer MoSe<sub>2</sub>,” *Phys. Rev. Lett.* **114**, 037401 (2015).

<sup>23</sup> Y. Li and et al., “Valley splitting and polarization by the Zeeman effect in monolayer MoSe<sub>2</sub>,” *Phys. Rev. Lett.* **113**, 266804 (2014).

<sup>24</sup> X. Xu, W. Yao, D. Xiao, and T. F. Heinz, “Spin and pseudospins in layered transition metal dichalcogenides,” *Nat. Phys.* **10**, 343–350 (2014).

<sup>25</sup> W. Yao, D. Xiao, and Q. Niu, “Valley-dependent optoelectronics from inversion symmetry breaking,” *Phys. Rev. B* **77**, 235406 (2008).

<sup>26</sup> D. Xiao, W. Yao, and Q. Niu, “Valley-contrasting physics in graphene: Magnetic moment and topological transport,” *Phys. Rev. Lett.* **99**, 236809 (2007).

<sup>27</sup> Z. Y. Zhu, Y. C. Cheng, and U. Schwingenschlögl, “Giant spin-orbit-induced spin splitting in two-dimensional transition-metal dichalcogenide semiconductors,” *Phys. Rev. B* **84**, 153402 (2011).

<sup>28</sup> D. Xiao, G.-B. Liu, W. Feng, X. Xu, and W. Yao, “Coupled spin and valley physics in monolayers of MoS<sub>2</sub> and other group-VI dichalcogenides,” *Phys. Rev. Lett.* **108**, 196802 (2012).

<sup>29</sup> M. Topsakal, E. Aktürk, and S. Ciraci, “First-principles study of two- and one-dimensional honeycomb structures of boron nitride,” *Phys. Rev. B* **79**, 115442 (2009).
